# Supplementary material for: Position-aware Graph Neural Networks
Source: arXiv:1906.04817 source file (2019-06-13)
Supplement: Supplementary file 1 [file 060appendix.tex]

\section{Appendix}

\begin{proof}

Proof of Proposition 1.

No pair of nodes have the same position-aware node embeddings, otherwise the two nodes have distance $0$ in the embedding space although their shortest path distance is $1$.
Since $f_p(v_i)$ is a function of $f_{s_q}(v_i)$, then no pair of nodes have the same structure-aware node embeddings as well.
If a pair of node have isomorphic $q$-hop neighbourhood graph, their each hop neighbour below $q$ is the same, thus the inputs for $f_{s_q}$ are the same, thus they should have the same structure-aware embeddings, which contradicts with the fact. Thus no pair of nodes have isomorphic $q$-hop neighbourhood graph.

On the reverse side, if no pair of nodes have isomorphic $q$-hop neighbourhood graph, then there exists $f_{s_q}$ such that each node has different structure-aware embeddings $f_{s_q}(v_i)$, because the inputs to $f_{s_q}$ are different.
Since each node have different position-aware embeddings $f_p(v_i)$, there exist an one-to-one mapping $g$ that maps each structure-aware embedding to corresponding position-aware embeddings.

\end{proof}

\begin{proof}
Proof of Proposition 2.
We propose a constructive proof.
Suppose such a function $g$ exist.
Then, we construct a new graph $G'$, via first independently construct $q+1$-hop neighbourhood graphs for each of the node in the original graph $G$, then take the union as $G'$.
Then, adding any edge between the neighbourhood graphs will not affect the structure-aware embedding method, yet it will change the shortest path distance between nodes in different neighbourhood graphs. This requires $g$ to map the same input to different outputs which conflicts with the definition of a function, therefore such $g$ does not exist.

\end{proof}

\begin{proof}
Proof of Proposition 3.

If two nodes have isomorphic $\infty$-hop neighbourhood graphs where $q$ is greater equal than the diameter of the graph, then for any anchor $S^l_1$ in $v_i$'s $\infty$-hop neighbourhood graph, there exists another anchor $S^l_2$ in $v_j$'s $\infty$-hop neighbourhood graph with $d_{sp}(v_i, S^l_1) = d_{sp}(v_j, S^l_2)$, thus the mapping is bijective. Therefore $d_{sp}(v_i, S^l)$ follows the same distribution and $p(d_{sp}(v_i, S^l)) = p(d_{sp}(v_j, S^l))$. Since the neighbours of $v_i$ and $v_j$ have isomorphic $\infty$-hop neighbourhood graphs as well, the statement holds true iteratively. 
If $p(d_{sp}(v_i, S^l)) = p(d_{sp}(v_j, S^l))$ iteratively, and the $q$-hop neighbourhood graphs of $v_i$ and $v_j$ are not $\infty$-hop isomorphic. Since the both neighbourhood graphs are defined over the same set of nodes, with out loss of generality, we assume that the non-isomorphism occurs such that node pairs $v_e, v_f$ in $v_i$'s neighbourhood graph are connected and $v_g, v_h$ in $v_j$'s neighbourhood graph are not. Then, $p(d_{sp}(v_e, S^l)) \neq p(d_{sp}(v_g, S^l))$ because $v_e$ has one more anchor ($v_f$) with distance one compared with $v_g$. Since $v_e$ and $v_g$ are within $v_i$ and $v_j$ neighbourhood graph respectively, $p(d_{sp}(v_i, S^l)) = p(d_{sp}(v_j, S^l))$ does not hold true iteratively, which conflicts with the assumption. Thus, the $q$-hop neighbourhood graphs of $v_i$ and $v_j$ are $\infty$-hop isomorphic, which finishes the proof.
\end{proof}
